# Supplementary material for: Steer'n Roll: A Stereoscopic Flow-Sensing Strategy for Planktonic Prey Detection and Capture
Source: arXiv:2601.20421 source file (2026-04-12)

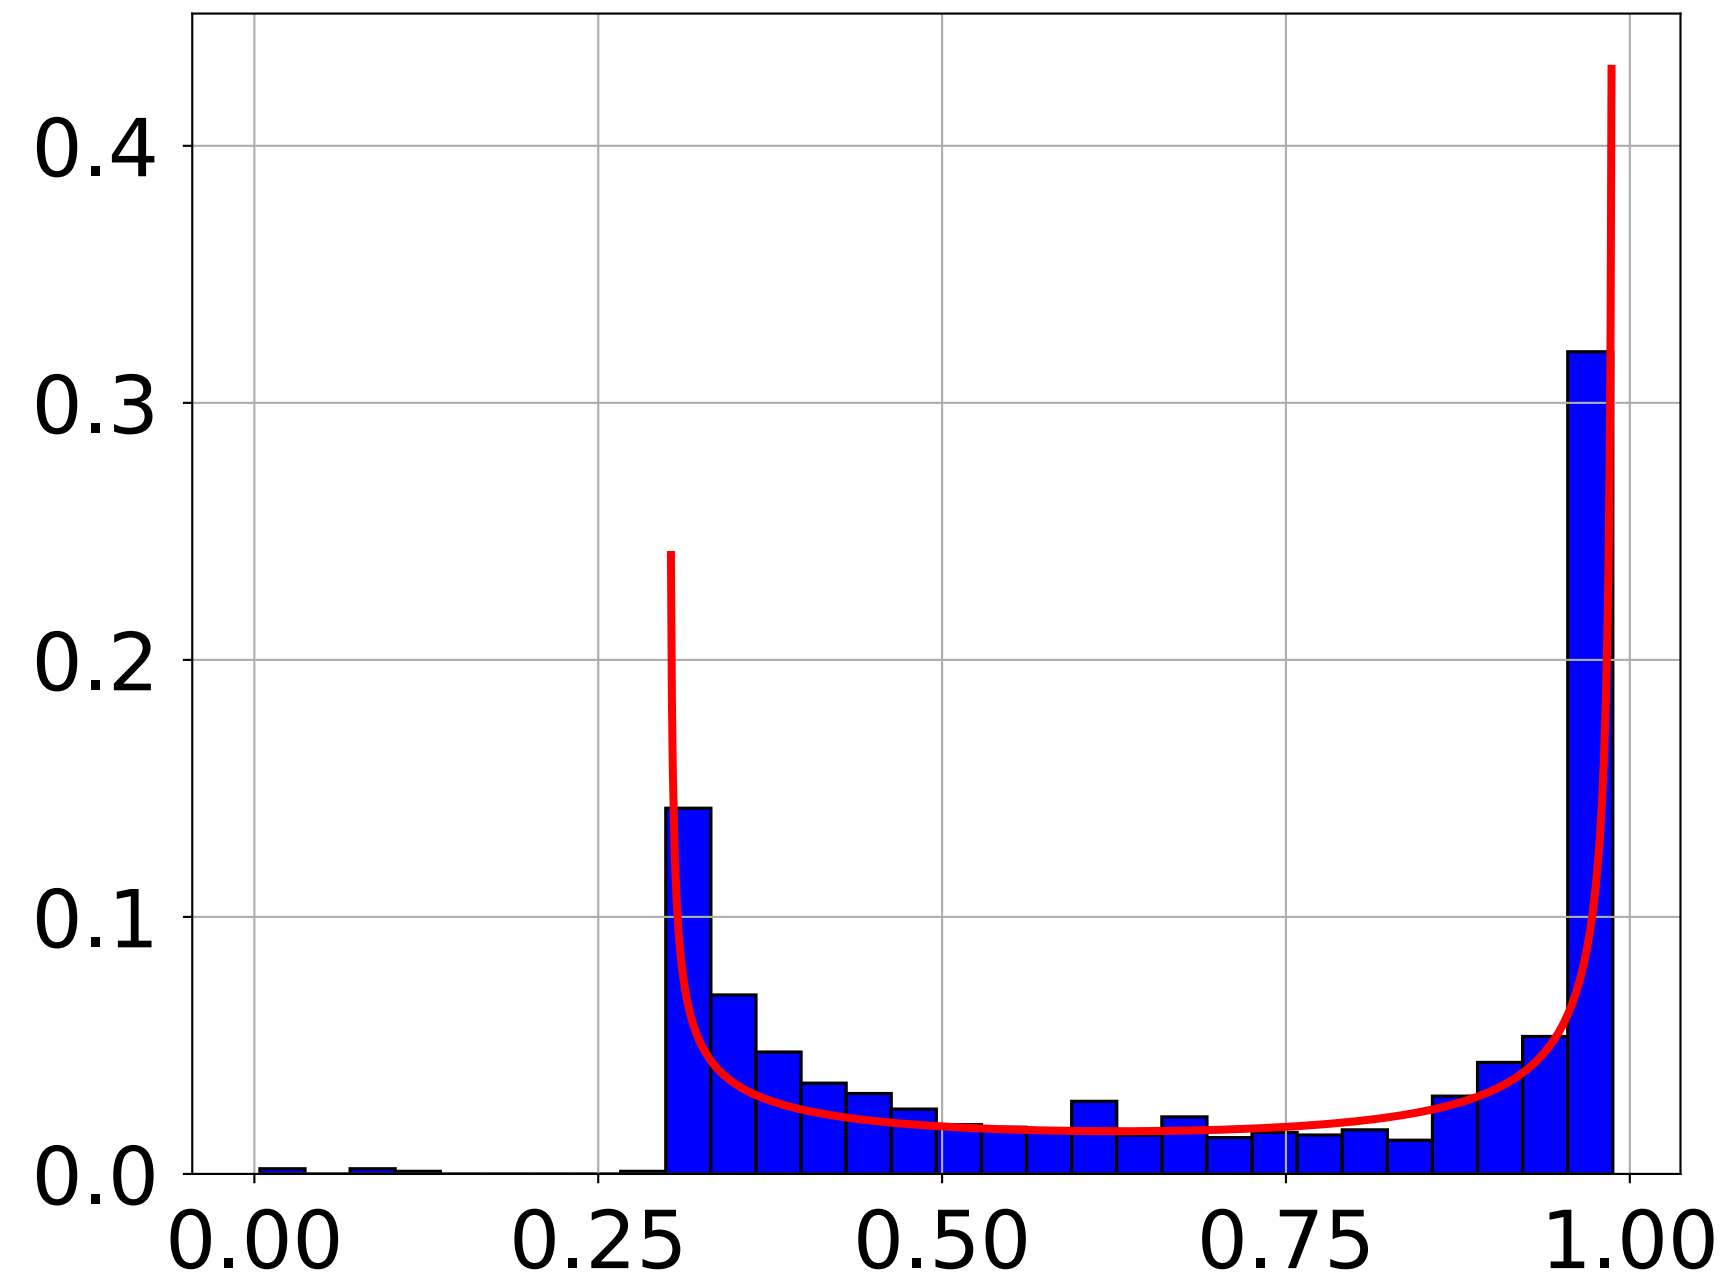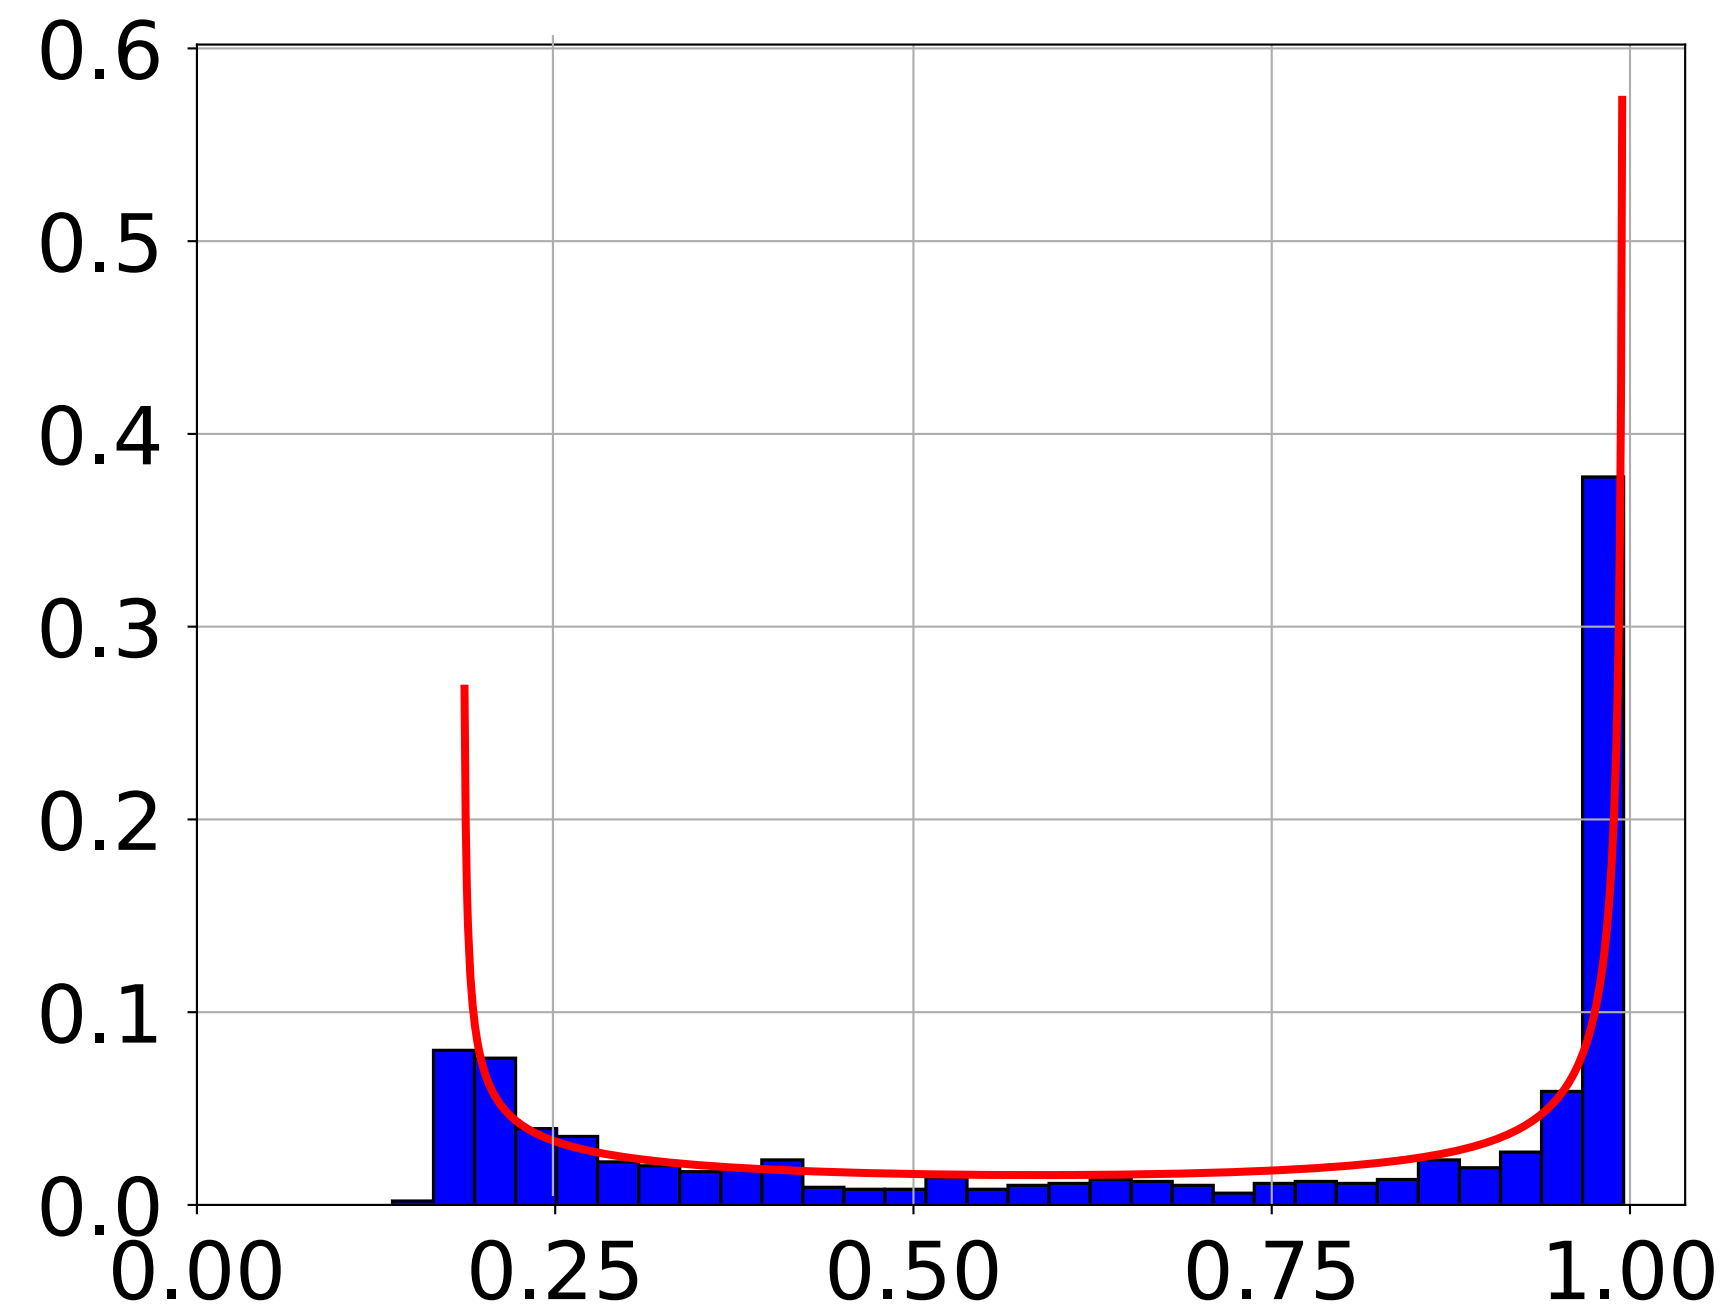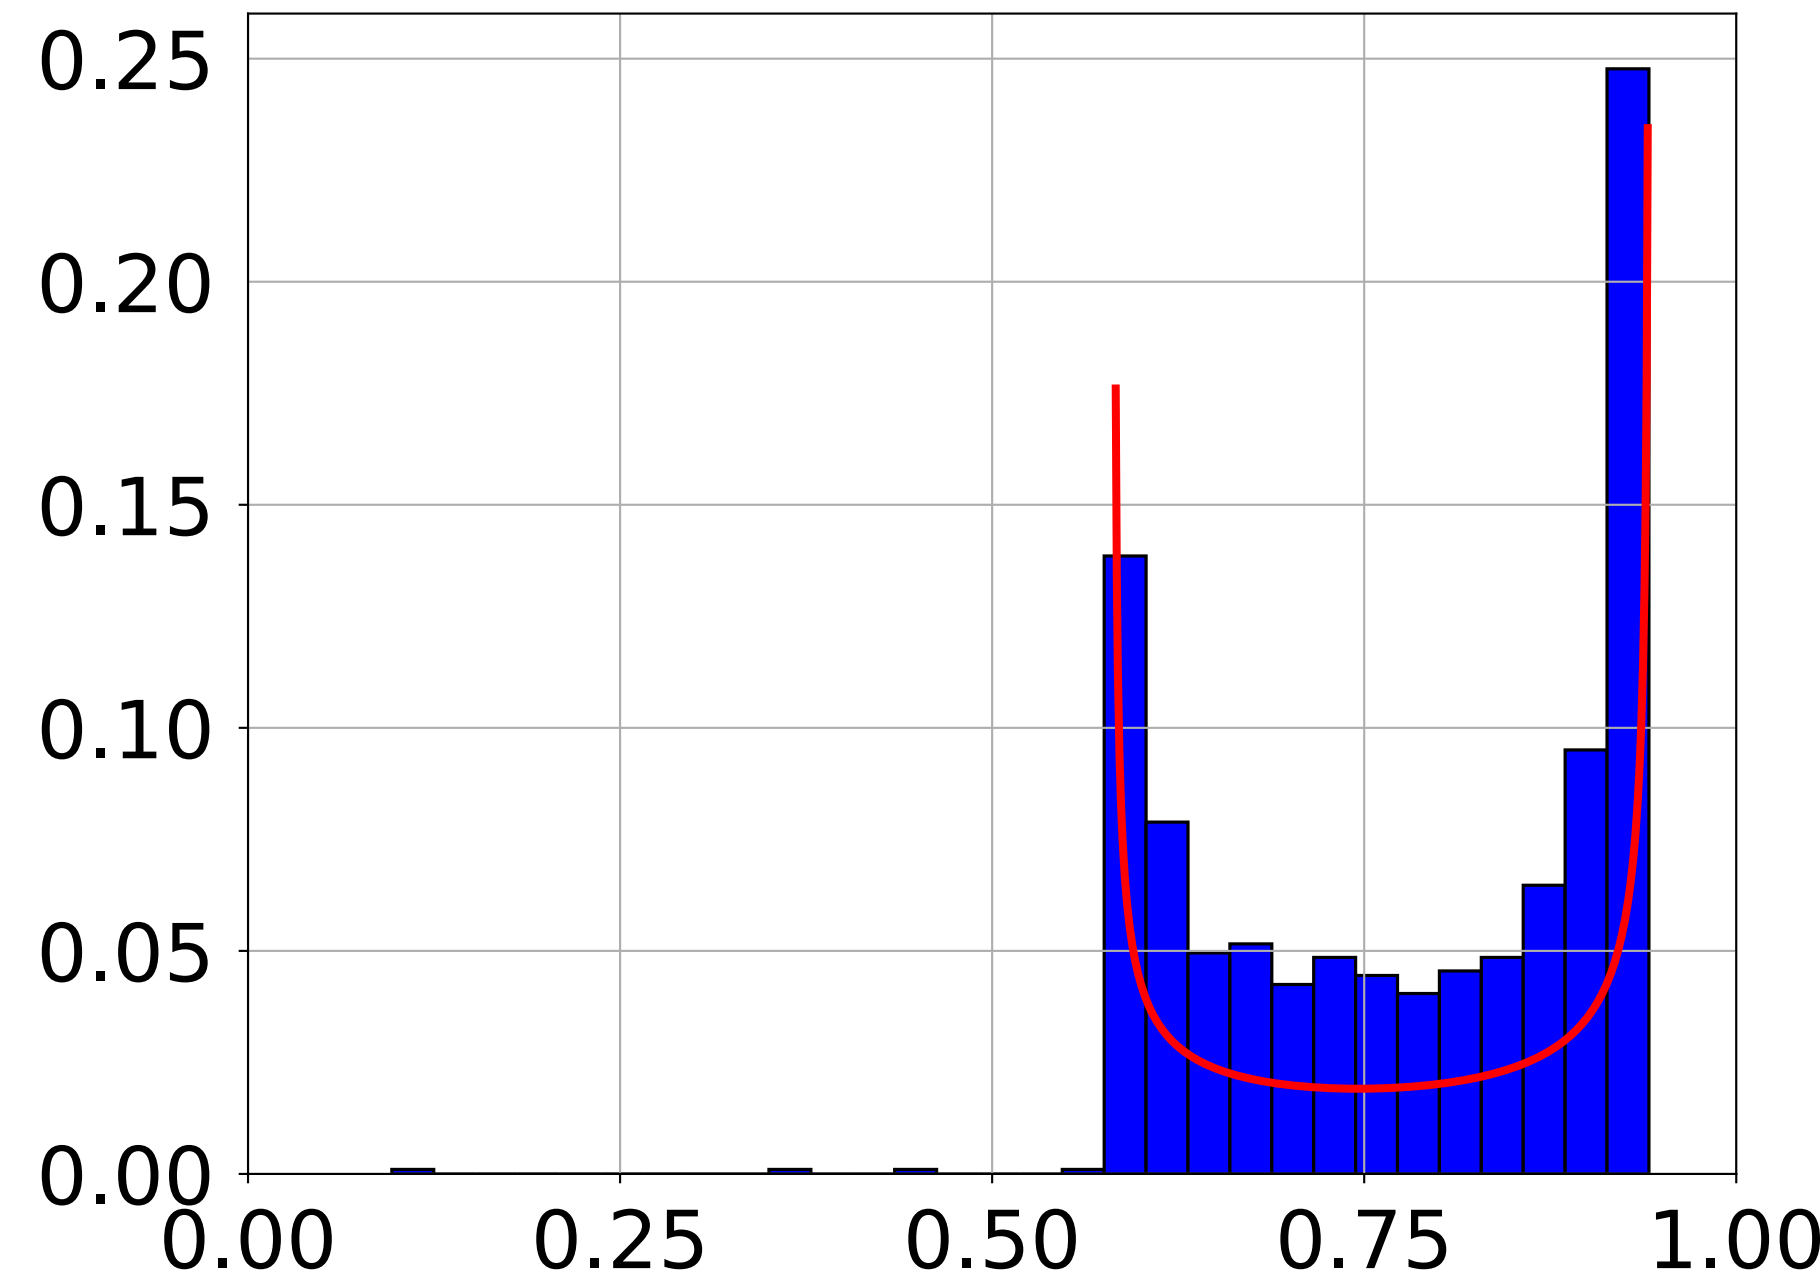

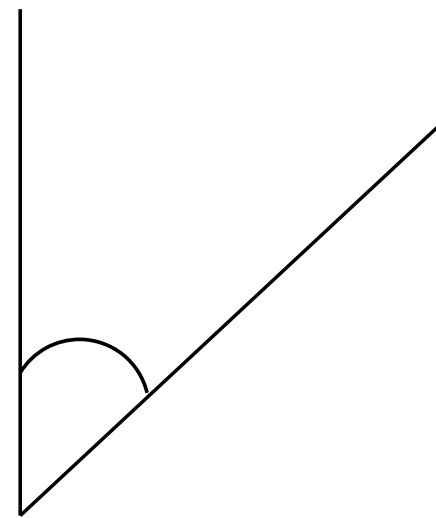

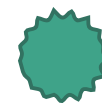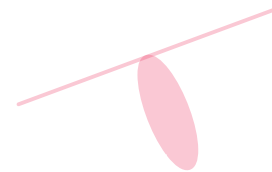

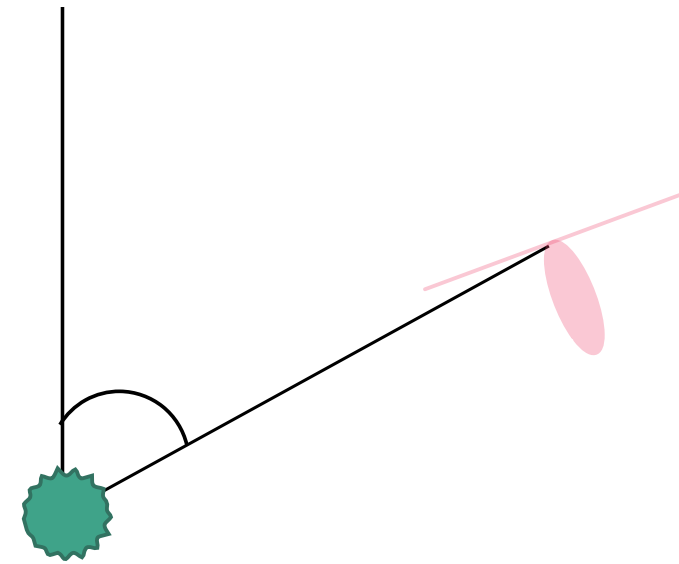

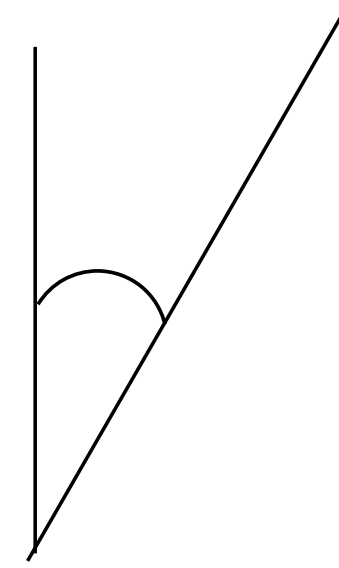

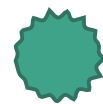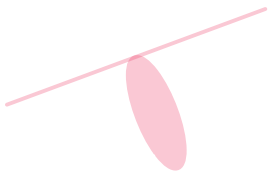

Supplement: Supplementary file 1 [file Fig_S4_suppl.pdf]
